# Supplementary material for: Efficient model predictive control for nonlinear systems modelled by deep neural networks
Source: arXiv:2405.10372 source file (2024-05-16)
Supplement: Supplementary file 1 [file appendix.tex]

\section{Neural Network Parameters}\label{sec:append}
The NN weights and biases used in Section \ref{subsec:sim1} are:
\begin{align}
	W_1 &= 
	\begin{bmatrix}
		0.6266 & 0.8433 & 0.3241 \\
		-0.2485 & -1.5838 & -0.5620 \\
		0.5243 & -1.4939 & 1.1992 \\
		-0.4300 & -1.4659 & 0.1102 \\
		0.2629 & 0.6789 & -1.2695
	\end{bmatrix}, ~
	b_1 = \begin{bmatrix}
		-1.0191 \\
		-1.3852\\
		0.9549\\
		-0.6011\\
		-1.1719
	\end{bmatrix}, \nonumber\\
	W_2 &= 
	\begin{bmatrix}
		-0.4617 & 0.6824 & 0.2419 & 0.0344 & 0.4333 \\
		-0.6691 & 0.3819 & 0.3326 & -0.7591 & -0.6569
	\end{bmatrix}, \nonumber\\
	b_2 &= \begin{bmatrix}
		-1.0719 \\
		-1.0741
	\end{bmatrix}. \nonumber
\end{align}

The NN weights and biases used in Section \ref{subsec:sim2} are:
\begin{align}
	W_1 &= 	
	\begin{bmatrix}
		-0.4222  & -0.0197 &  -2.0321  &  1.5436 &  -0.4479 \\
		1.9507   &  0.0910 &  -0.7421  & -0.8413 &   0.4752 \\
		-1.0388  & -0.0485 &   0.8895  &  0.1275 &  -0.4584 \\
		0.4240   & 0.0198  & -0.2903   & -0.0492 &  -0.3834 \\
		0.0765   & 0.0036  & -0.1093   & 0.1257  & -0.2643 \\
		-0.0261  & -0.0012 &   0.0683  & -0.0027 &  -0.3298 \\
		-0.2489  & -0.0116 &  -0.2231  &  0.2467 &  -1.6979 \\
		-0.2920  & -0.0136 &  -0.0946  &  0.1167 &   0.5676 \\
		0.0057   & 0.0003  &  0.5001   & -0.2043 &   0.0171 \\
		-0.2088  & -0.0097 &   1.2994  &  -0.7251 &   0.5568 \\
		0.3301   & 0.0154  & -0.1541   & -0.1234  & -0.0113 \\
		-0.3912  & -0.0183 &  -1.3695  &  1.0931 &  -0.3167 \\
		0.0230   & 0.0011  & -0.2048   & 0.1767  &  2.1451 \\
		0.1544   & 0.0072  & -0.5275   & 0.2610  & -0.0524 \\
		-0.4265  & -0.0199 &  -0.0092  &  0.0665 &  -0.4478 \\
		-0.0057  & -0.0003 &  -0.1715  & -0.0136  &  0.2887 \\
		0.4578   & 0.0214  & -0.2018   &-0.1380  & -1.1072 \\
		-0.0798  & -0.0037 &  -0.0479  & -0.0048 &   0.0212 \\
		0.0910   & 0.0042  &  0.2241   & 0.0222 &  -0.2237 \\
		0.0298   & 0.0014  &  0.1805   & 0.1418 &  -0.4708 
	\end{bmatrix}, \nonumber\\
	W_2 &= 
	\begin{bmatrix}
		-1.3682 \\ 1.5483 \\ 0.6767\\ -0.2115\\ -1.0598\\ -0.1589\\ -0.1682\\ -0.3634\\ -0.4160\\ -1.9243\\ -0.9446\\
		1.7470\\ 0.3930\\ -0.4689\\ 0.0031\\ 0.1921\\ -0.6993\\ 0.5137\\ -0.7177\\ 0.2741
	\end{bmatrix}^\top, 
	b_1 = 
	\begin{bmatrix}
		-6.3445 \\
		8.6755 \\
		-2.7326 \\
		-1.5149 \\
		-6.3206 \\
		6.4377 \\
		2.1055 \\
		4.3617 \\
		-2.4270 \\
		5.8466 \\
		0.4227 \\
		-2.9681 \\
		-3.2292 \\
		2.3160 \\
		1.9494 \\
		-2.2767 \\
		-1.9752 \\
		1.9222 \\
		-0.2966 \\
		2.8062 
	\end{bmatrix},~
	b_2 = -0.7311.
	\nonumber
\end{align}
